# Supplementary material for: A Diamagnetic Trap with 1D Camelback Potential
Source: arXiv:1405.5220 ancillary file (2014-05-22)
Supplement: Supplementary file 1 [file MAGTRAP-SuppMat.pdf]

# SUPPLEMENTARY INFORMATION:

# A Diamagnetic Trap with 1D Camelback Potential

Oki Gunawan[1]*, Yudistira Virgus[1,2]

[1] IBM T. J. Watson Research Center, Yorktown Heights, NY 10598

[2] College of William and Mary, Williamsburg, VA 23187

*Correspondence to: ogunawa@us.ibm.com.

## Outline:

**I. Materials and Method**
- A. Materials
- B. Method

**II. Supplementary Text**
- A. Magnetic Field Calculation
  - A.1 Exact calculation: Scalar potential model.
  - A.2 Exact calculation: Vector potential/Surface current model.
  - A.3 Analytical approximation at center plane: Parallel Dipole Line model
  - A.4 Comparison of various models
- B. The Magnetization of the Rod
- C. The Vertical (*y*) Confinement
- D. The Longitudinal (*z*) Confinement (Camelback Potential)
- E. The Lateral (*x*) Confinement and Comparison
- F. The Oscillation in the Camelback Potential
- G. Underdamped Oscillation Analysis
- H. Custom-Designed 1D Potential System

**References**

# I. MATERIALS AND METHOD

## A. Materials

In this study we used two magnetic trap setups with different aspect ratio *L*/*a* as shown below:

| Setup name | Magnet radius $a$ (mm) | Magnet length $L$ (mm) | Magnetization $M$ ($10^6$ A/m) |
|---|---|---|---|
| **"*L*/*a* = 8"** | 3.15 ± 0.05 | 25.4 ± 0.05 | 1.11 ± 0.04 |
| **"*L*/*a* = 4"** | 3.15 ± 0.05 | 12.6 ± 0.05 | 0.97 ± 0.04 |

**Table S1.** Magnetic trap parameters.

The magnets are diametrically magnetized made of neodymium iron boron (NIB) with similar magnetization. The magnetization $M$ is determined from the far field magnetic field data in the dipole limit (Eq. 18) as shown in Figure S3. The magnetic field is measured with calibrated Lakeshore 410 Gaussmeter (Sensor calibration# 787).

For the graphite rods we use mechanical pencil leads (Pentel) with hardness type "HB" and various nominal diameters (0.3, 0.5, 0.7 and 0.9 mm). We label the graphite rod sample, for example, as "HB/0.5" to indicate the hardness type of HB and *nominal* diameter of 0.5 mm. The actual diameters are slightly different than the nominal diameter. We measure the actual diameters using digital caliper and report them in Table S2.

## B. Method

To investigate the motion dynamics of the trapped graphite rod in our diamagnetic trap we set up the system as shown in Figure S1a. A glass enclosure (a round beaker) is necessary to eliminate air agitation effect – as we found that the graphite rod could develop random movement due to surrounding air agitation as the confinement of the camelback potential is very weak. The experiment can also be done in a vacuum cryostat to reduce the air friction effect as discussed in Section II.G.

We use standard stopwatch to measure most of the oscillation periods. To capture the detailed oscillatory motion of the graphite rod along the camelback potential, we use video capture (USB video camera Dino-Lite AD-7013MZT) followed by image processing routine developed using MATLAB. The method is illustrated in Figure S1b. First we capture the oscillation video, establish an "inspection line" along the rod trajectory ($z$-axis) and extract the pixel intensity as shown in the upper panel of Figure S1b. We pick a pixel intensity value that serves as the "edge threshold" to determine the edge's coordinate of the graphite rod (indicated as solid circle). We repeat this process for every video frame to obtain the oscillation plot as shown in Fig. 3a and Figure S11. Note that the

actual frame rate (FR) of the video is slightly different than the specified FR. Thus it is necessary to calibrate the FR by capturing a video of a running stopwatch. The actual FR is used to calculate the timestamp of each image.

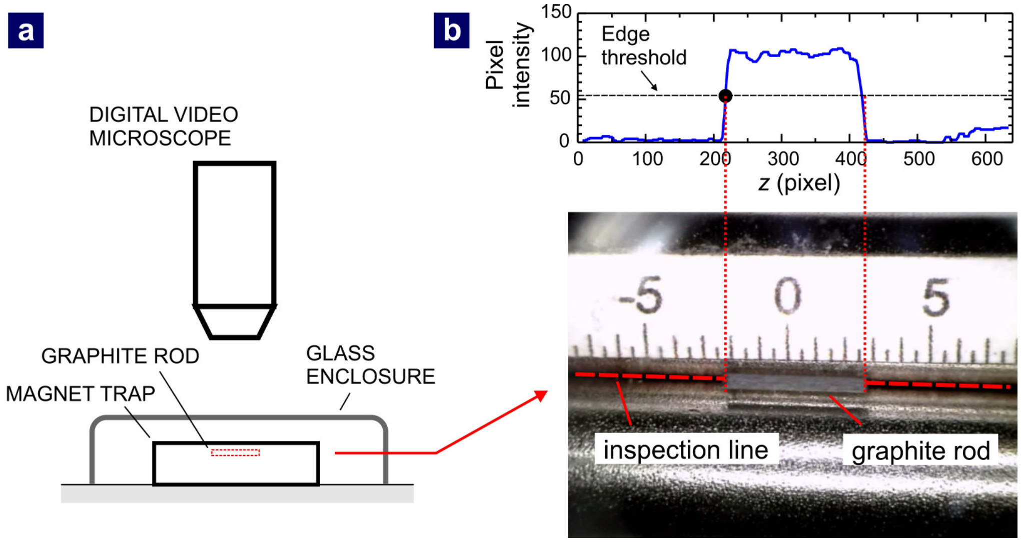


**Figure S1. Experimental setup and oscillation analysis.** (**a**) The setup. (**b**) Example of video capture and motion detection analysis.

An example of a raw video footage of the oscillation is shown in Supplementary Information Movie S1. The video is for magnet setup "*L*/*a*=8" and graphite rod HB/0.5 with length $l$ = 4.5 mm. The calibrated actual frame rate is 15.828 frame/sec, instead of the specified 15 frame/sec. The oscillation data extracted from this video is plotted in Fig. 3a.

# II. SUPPLEMENTARY TEXT

## A. Magnetic Field Calculation

We present three calculation models for the magnetic field distribution of the diametric magnet as illustrated in Figure S2:

**(1) Exact calculation: Scalar potential model.**
Provides a compact, exact expression that can be easily implemented numerically.

**(2) Exact calculation: Vector potential/Bound surface current model.**
More intuitive model but more lengthy. Provides insight to the origin of the "camelback hump".

**(3) Analytical approximation at center plane: Parallel Dipole Line (PDL) model**
Provides closed-form expression and good approximation at the center of the trap ($x = 0$, $z \sim 0$). It simplifies the analysis of the stability condition and longitudinal oscillation of the graphite rod.

In this work we refer the first two models as "Exact" models and the last one as "PDL" model.

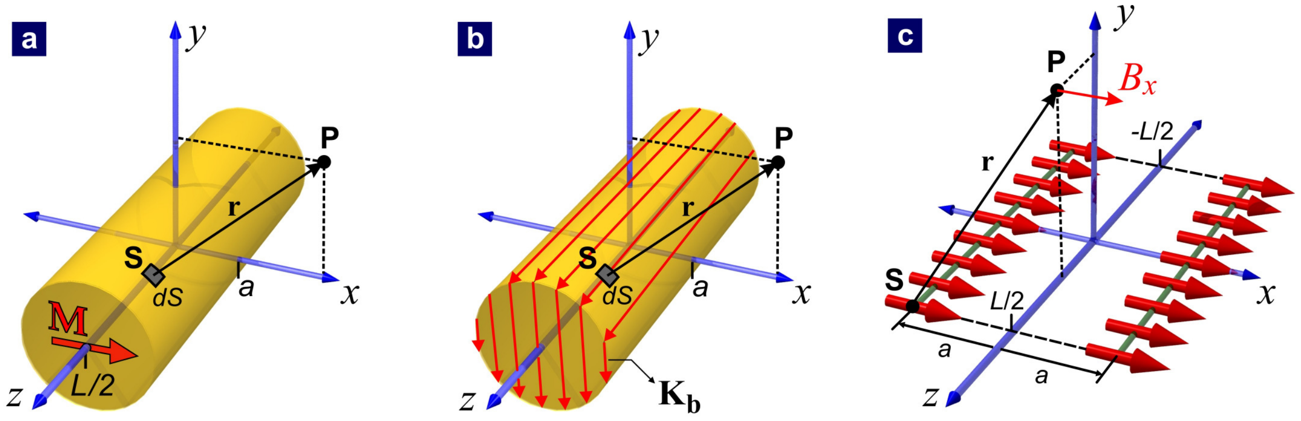


**Figure S2. Magnetic field calculation models**: (**a**) Magnetic scalar potential model of one magnet. (**b**) Magnetic vector potential or bound surface current model of one magnet. The surface currents $\mathbf{K_B}$ are indicated as red arrows. (**c**) Parallel Dipole Line (PDL) model for a pair of magnets.

### A.1 Exact Calculation: Magnetic Scalar Potential Model

Here we derive the exact magnetic field expression due to a cylindrical diametric magnet with a uniform volume magnetization $\mathbf{M}$ along $x$-axis using magnetic scalar potential $\Phi_M$ where $\mathbf{H} = -\nabla\Phi_M$ with $\mathbf{H}$ is the magnetic field intensity. This scalar potential can be written as (Ref. [24], Chapter 5.10):

$$\Phi_M = \frac{1}{4\pi}\left[-\int_V \frac{\nabla\cdot\mathbf{M}}{r}dV + \oint_S \frac{\hat{\mathbf{n}}\cdot\mathbf{M}}{r}dS\right] \tag{10}$$

In the case of uniform magnetization throughout the volume *V*, the first term vanishes. Consider a surface element *dS* at point **S** = [$x_S$, $y_S$, $z_S$] (written in Cartesian vector form [*x*, *y*, *z*]) as shown in Figure S2a. In cylindrical coordinates, we have: $x_S = a\cos\phi$, and $y_S = a\sin\phi$. This surface element contributes to the scalar potential at position $\mathbf{P} = [x, y, z]$ with a relative position vector:

$$\mathbf{r} = \mathbf{P} - \mathbf{S} = [x - a\cos\phi, y - a\sin\phi, z - z_S] \tag{11}$$

The surface element can be written as: $dS = a\,d\phi dz_S$. In this model, due to the term $\hat{\mathbf{n}}\cdot\mathbf{M}$, only the sheath contributes to the magnetic scalar potential which can be calculated as:

$$\Phi_M = \frac{M\,a}{4\pi}\int_0^{2\pi}\int_{-L/2}^{L/2}\frac{\cos\phi}{\sqrt{(x-a\cos\phi)^2+(y-a\sin\phi)^2+(z-z_S)^2}}dz_S d\phi \tag{12}$$

We can solve the first integral with substitution: $u = z - z_S$ and $s^2 = (x - a\cos\phi)^2 + (y - a\sin\phi)^2$ :

$$\int du/\sqrt{u^2+s^2} = \ln(u + \sqrt{u^2+s^2}) \tag{13}$$

Unfortunately, the second integral has no analytical solution. Now we have:

$$\Phi_M = \frac{M\,a}{4\pi}\int_0^{2\pi}\ln\left[\frac{u_1+\sqrt{u_1^{\,2}+s^2}}{u_2+\sqrt{u_2^{\,2}+s^2}}\right]\cos\phi d\phi = -\frac{M\,a}{4\pi}\int_0^{2\pi}\sum_{n=1,2}(-1)^n\ln(u_n+\sqrt{u_n^{\,2}+s^2})\cos\phi d\phi \tag{14}$$

where $u_1 = z + L/2$ and $u_2 = z - L/2$.

We now can calculate the magnetic field given as $\mathbf{B} = -\mu_0\nabla\Phi_M$. Note that the gradient operator is calculated with respect to the position variable *x*, *y*, *z* at point **P**. We use substitution $f(x, y, z) = \ln(u + \sqrt{u^2+s^2})$ and we have the gradient (in Cartesian vector form):

$$\nabla f(x, y, z) = \frac{[x - a\cos\phi,\ y - a\cos\phi,\ u + \sqrt{u^2+s^2}]}{u^2 + s^2 + u\sqrt{u^2+s^2}} \tag{15}$$

Finally we obtain the magnetic field due the magnet:

$$\mathbf{B}_M(x,y,z) = \frac{\mu_0 Ma}{4\pi}\int_0^{2\pi}\sum_{n=1,2}\frac{(-1)^n}{u_n^{\,2}+s^2+u_n\sqrt{u_n^{\,2}+s^2}}\begin{bmatrix} x-a\cos\phi \\ y-a\cos\phi \\ u_n+\sqrt{u_n^{\,2}+s^2}\end{bmatrix}\cos\phi\, d\phi \quad (16)$$

where $s^2=(x-a\cos\phi)^2+(y-a\sin\phi)^2$ and $u_1=z+L/2$ and $u_2=z-L/2$.

**Far field limit:**

A useful and simple expression can be obtained at far field limit along the magnetization direction ($x$-axis) where the magnetic field approaches the dipole limit. Here we have: $y = 0$, $z = 0$, $x \gg L$ and $x \gg a$ and Eq. 16 can be simplified to:

$$B_x(x,0,0) = \frac{\mu_0 M\,a}{4\pi}\int_0^{2\pi}\cos\phi(x-a\cos\phi)\frac{L\sqrt{s^2+(L/2)^2}}{[s^2+(L/2)^2]s^2}d\phi \quad (17)$$

$$\simeq \frac{\mu_0 M\,a}{4\pi}\int_0^{2\pi}\cos\phi(x-2a\cos\phi)\frac{L}{x^3}d\phi = \frac{\mu_0 M\,a^2 L}{2\,x^3} \quad (18)$$

Note that this result could also be alternatively derived directly from a magnetic dipole expression: $\mathbf{B}=\mu_0/4\pi\times[3(\hat{\mathbf{r}}\cdot\mathbf{m})\hat{\mathbf{r}}-\mathbf{m}]/r^3$ (Ref. [25], pg. 246) and using the relationship: $\mathbf{m}=\pi a^2 L M\,\hat{\mathbf{x}}$. This far field, pure dipole limit characteristics is used to extract the value of $M$ from the long distance segment of the experimental data as shown in Figure S3.

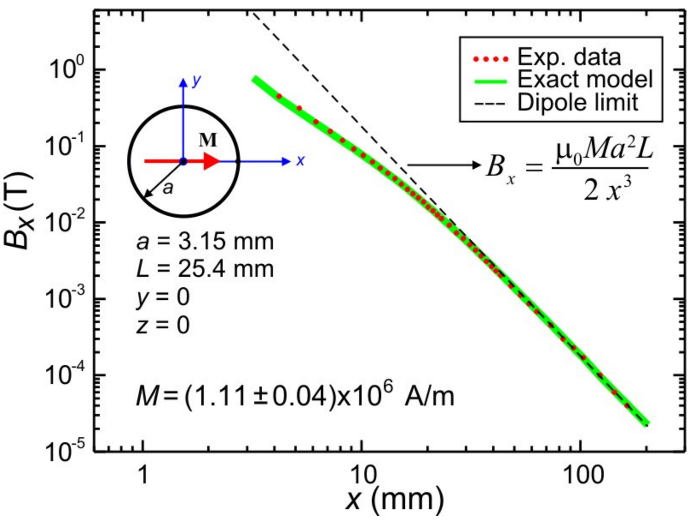


**Figure S3. Magnetic field of a diametric magnet: theory and experiment**. Field is calculated along $x$ direction using "Exact" calculation (scalar potential) model. The dipole limit at long distance data can be used to extract $M$.

**Comparison with experimental data:**

The “Exact” magnetic field expression derived in Eq. 16 can be compared with the experimental data of a diametric magnet ($a$ = 3.15 mm, $L$ = 25.4 mm). The data is presented in Figure S3 which shows a very good agreement. The value of the magnetization $M$ can be obtained from the pure dipole limit at long distance asymptote or using curve fitting to the “Exact” model with $M$ as a single independent parameter.

## *A.2 Exact Calculation: Magnetic Vector Potential/Bound Surface Current Model*

Here we present an alternative calculation using magnetic vector potential or bound surface current model that produces the same result as the scalar potential model (Section II.A.1). The advantage of this model is that we can decompose separate contributions of the bound current from the sheath and faces part of the cylindrical magnet to investigate the origin of the camelback potential.

We first calculate the magnetic vector potential $\mathbf{A}$ at any point P in space where $\mathbf{P}=[x,y,z]$ and then calculate the magnetic field $\mathbf{B}$ using: $\mathbf{B}=\nabla\times\mathbf{A}$. We consider a single diametric cylindrical magnet as shown in Figure S2b with radius $a$ and length $L$. The magnetic vector potential $\mathbf{A}$ due to a permanent magnet with volume magnetization $\mathbf{M}(\mathbf{r})$ is given as (Ref. [25], Pg. 264):

$$\mathbf{A}=\frac{\mu_0}{4\pi}\left[\int_V \frac{\mathbf{J}_b}{r}dV+\oint_S \frac{\mathbf{K}_b}{r}dS\right] \quad (19)$$

where $\mathbf{J}_b=\nabla\times\mathbf{M}$ is the bound current within the magnet and $\mathbf{K}_\mathrm{b}=\mathbf{M}\times\hat{\mathbf{n}}$ is the bound surface current on the magnet surface where $\hat{\mathbf{n}}$ is the unit vector normal to the surface. Since the magnetization is constant and uniform, $\mathbf{J}_\mathrm{b}$ = 0 everywhere and the contribution to the vector potential comes only from the bound surface current. The distribution of the surface current is shown in Figure S2b. We can separate the magnetic field calculation into two parts: (1) the sheath and (2) the two flat faces at the magnet ends.

### A.2.a Magnetic field due to the sheath surface ($B_S$)

We will first calculate the magnetic vector potential due to the distribution of the bound surface current on the magnet sheath. The normal surface unit vector of the sheath is given as: $\hat{\mathbf{n}}=\cos\phi\hat{\mathbf{x}}+\sin\phi\hat{\mathbf{y}}$. Using $\mathbf{K}_\mathrm{b}=\mathbf{M}\times\hat{\mathbf{n}}$, the bound surface current on the sheath due to magnetization $\mathbf{M}=M\,\hat{\mathbf{x}}$ is: $\mathbf{K}_\mathrm{b}=M\sin\phi\hat{\mathbf{z}}$ which points towards $z$+ for the upper half ($0<\phi<\pi$) and towards $z$- for the lower half of the sheath ($\pi<\phi<2\pi$).

Consider a surface element d$S$ at point $\mathbf{S}(x_S, y_S, z_S)$. In the cylindrical coordinates, we have: $x_S=a\cos\phi$, and $y_S=a\sin\phi$. This surface element contributes to the magnetic field vector potential $\mathbf{A}_S$ at position $\mathbf{P}$ with a relative position vector as described in Eq. 11. The surface element can be written as: $dS=a\,d\phi\,dz_S$. The magnetic vector potential can be calculated as:

$$\mathbf{A}_S(\mathbf{r}) = \hat{\mathbf{z}}\frac{\mu_0 M\, a}{4\pi}\int_0^{2\pi}\int_{-L/2}^{L/2}\frac{\sin\phi}{\sqrt{(x-a\cos\phi)^2+(y-a\sin\phi)^2+(z-z_S)^2}}dz_S d\phi \tag{20}$$

Using the same integral and substitution in Eq. 13, we can solve one of the two integrals:

$$\begin{aligned}\mathbf{A}_S(\mathbf{r}) &= \hat{\mathbf{z}}\frac{\mu_0 M\, a}{4\pi}\int_0^{2\pi}\ln\left[\frac{u_1+\sqrt{u_1^{\,2}+s^2}}{u_2+\sqrt{u_2^{\,2}+s^2}}\right]\sin\phi\, d\phi \\ &= \hat{\mathbf{z}}\frac{\mu_0 M\, a}{4\pi}\int_0^{2\pi}\sum_{n=1,2}(-1)^{n+1}\ln(u_n+\sqrt{u_n^{\,2}+s^2})\sin\phi\, d\phi\end{aligned} \tag{21}$$

where $u_1 = z + L/2$ and $u_2 = z - L/2$.

We now can calculate the magnetic field due to the sheath surface using: $\mathbf{B} = \nabla\times\mathbf{A}_S$ where $\mathbf{A}_S = \mathrm{A}_z\,\hat{\mathbf{z}}$ , that yields: $\mathbf{B}_S = [\partial \mathrm{A}_z/\partial y,\ -\partial \mathrm{A}_z/\partial x,\ 0]$. Note that the derivative is calculated with respect to the position variable *x*, *y*, *z* at point **P** (see Eq. 15).

Finally, the magnetic field due to the sheath (in Cartesian vector form) is:

$$\mathbf{B}_S(x,y,z) = \frac{\mu_0 M\, a}{4\pi}\int_0^{2\pi}\sin\phi\sum_{n=1,2}\frac{(-1)^{n+1}}{s^2+u_n^{\,2}+u_n\sqrt{s^2+u_n^{\,2}}}\begin{bmatrix} y-a\sin\phi \\ -x+a\cos\phi \\ 0\end{bmatrix}d\phi \tag{22}$$

where $s^2 = (x-a\cos\phi)^2+(y-a\sin\phi)^2$ and $u_{1,2} = z \pm L/2$.

### A.2.b Magnetic field due to the flat faces ($B_F$)

We now calculate the magnetic field contribution due to the two flat faces on the end of the magnet. The elemental surface on the faces is: $dS = dx_S dy_S$ , and the position vector from the surface element is: $\mathbf{r} = \mathbf{P} - \mathbf{S} = [x - x_S, y - y_S, z - z_m]$, where $z_m$ corresponds to the flat surface at: $z_1 = -L/2$ and $z_2 = L/2$. The normal vectors of the surface are: $\hat{\mathbf{n}}_1 = -\hat{\mathbf{z}}$ and $\hat{\mathbf{n}}_2 = \hat{\mathbf{z}}$ for the two faces.

Using $\mathbf{K}_\mathrm{b} = \mathbf{M}\times\hat{\mathbf{n}}$, the bound surface current on the flat faces are: $\mathbf{K}_{b1} = \mathrm{M}\,\hat{\mathbf{y}}$ and $\mathbf{K}_{b2} = -\mathrm{M}\,\hat{\mathbf{y}}$ for face #1 and #2 respectively. We use a Cartesian coordinate system because the magnetic field vector **A** only has *y* component.

Using Eq. 19:

$$\mathbf{A}_{Fm} = -(-1)^m \frac{\mu_0 M}{4\pi} \hat{\mathbf{y}} \int_{-a}^{a} \int_{-\sqrt{a^2 - x_S^2}}^{\sqrt{a^2 - x_S^2}} \frac{dy_S \, dx_S}{\sqrt{(x - x_S)^2 + (y - y_S)^2 + (z - z_m)^2}} \tag{23}$$

where the subscript $m$ is 1 or 2 for the two end faces (Figure S2b). We use substitution:

$$v = y - y_S \qquad \text{and} \qquad q_m^{\ 2} = (x - x_S)^2 + (z - z_m)^2 \tag{24}$$

Solving the integral with respect to $v$ by using the integral in Eq. 13:

$$\begin{aligned} \mathbf{A}_{Fm} &= \hat{\mathbf{y}} (-1)^m \frac{\mu_0 M}{4\pi} \int_{-a}^{a} \ln \left( \frac{v_2 + \sqrt{q_m^{\ 2} + v_2^{\ 2}}}{v_1 + \sqrt{q_m^{\ 2} + v_1^{\ 2}}} \right) dx_S \\ &= \hat{\mathbf{y}} (-1)^m \frac{\mu_0 M}{4\pi} \int_{-a}^{a} \sum_{n=1,2} (-1)^n \ln(v_n + \sqrt{q_m^{\ 2} + v_n^{\ 2}}) \, dx_S \end{aligned} \tag{25}$$

where $v_1 = y + \sqrt{a^2 - x_S^{\ 2}}$ and $v_2 = y - \sqrt{a^2 - x_S^{\ 2}}$. The total magnetic vector potential due to two end faces is simply $\mathbf{A}_F = \mathbf{A}_{F1} + \mathbf{A}_{F2}$.

The magnetic field at point **P** is $\mathbf{B} = \nabla \times \mathbf{A}$ where $\mathbf{A} = \mathrm{A}_F \, \hat{\mathbf{y}}$. This yields: $\mathbf{B}_F = [-\partial \mathrm{A}_F / \partial z, 0, \partial \mathrm{A}_F / \partial x]$ where the derivative calculation is similar to Eq. 15.

The magnetic field due to the flat faces is:

$$\mathbf{B}_F(x, y, z) = \frac{\mu_0 M}{4\pi} \sum_{m=1,2} (-1)^m \int_{-a}^{a} \sum_{n=1,2} \frac{(-1)^n}{v_n^{\ 2} + q_m^{\ 2} + v_n \sqrt{v_n^{\ 2} + q_m^{\ 2}}} \begin{bmatrix} -z + z_m \\ 0 \\ x - x_S \end{bmatrix} dx_S \tag{26}$$

where $v_{1,2} = y \pm \sqrt{a^2 - x_S^{\ 2}}$, $q_m^{\ 2} = (x - x_S)^2 + (z - z_m)^2$ and $z_{1,2} = \mp L/2$.

Finally the total magnetic field of a diametric magnet due to the sheath (Eq. 22) and the faces (Eq. 26) is given as:

$$\mathbf{B}_M(x, y, z) = \mathbf{B}_S(x, y, z) + \mathbf{B}_F(x, y, z) \tag{27}$$

### *A.3. Parallel Dipole Line (PDL) model: Analytical approximation at the trap center*

The models described in previous sections (A.1 and A.2) contain integral with no analytical solution thus requiring numerical integration. Here we describe Parallel Dipole Line (PDL) model that provides a good analytical approximation for the magnetic field at the center of the trap ($x$ = 0, $z$ ~ 0). *For an infinitely long diametric magnet the magnetic field around the center is exactly that of a distribution of magnetic dipole along the longitudinal axis.* In this model we have a distribution of magnetic dipoles along two parallel lines located at $x = \pm a$ and $z$ = -$L$/2 to $L$/2 as shown in Figure S2c.

Using the magnetic dipole field expression: $\mathbf{B} = \mu_0 / 4\pi \times [3(\hat{\mathbf{r}}\cdot\mathbf{m})\hat{\mathbf{r}} - \mathbf{m}]/r^3$ (Ref. [25], pg. 246) we can calculate the magnetic field at point **P** due to a magnetic dipole element $d\mathbf{m}$ at point **S** ($a$, 0, $z_S$):

$$d\mathbf{B} = d\mathbf{B}_2 + d\mathbf{B}_1 \quad \text{where} \quad d\mathbf{B}_1 = -\frac{\mu_0}{4\pi}\frac{d\mathbf{m}}{r^3} \quad \text{and} \quad d\mathbf{B}_2 = \frac{\mu_0}{4\pi}\frac{3(\hat{\mathbf{r}}\cdot d\mathbf{m})\hat{\mathbf{r}}}{r^3} \tag{28}$$

with $d\mathbf{m} = M\,\pi a^2 d z_S\,\hat{\mathbf{x}}$ and $\mathbf{r} = \mathbf{P} - \mathbf{S} = [a,\ y,\ z - z_S]$.

Note that due to symmetry of the trap system, the magnetic field at the center of the trap ($x$ = 0) would only have $x$-component ($B_y$ and $B_z$ are zero) and it will be *doubled* due to two dipole lines at $x = \pm a$.

The first term yields:

$$\mathbf{B}_{T,1}(y,z) = -\frac{\mu_0 M a^2}{2}\int_{-L/2}^{L/2}\frac{dz_S}{[a^2 + y^2 + (z - z_S)^2]^{3/2}}\hat{\mathbf{x}} \tag{29}$$

$$\mathbf{B}_{T,1}(y,z) = -\frac{\mu_0 M\,a^2}{2(y^2 + a^2)}\left(\frac{L/2 - z}{\sqrt{(L/2 - z)^2 + y^2 + a^2}} + \frac{L/2 + z}{\sqrt{(L/2 + z)^2 + y^2 + a^2}}\right)\hat{\mathbf{x}} \tag{30}$$

For the second term we have $(\hat{\mathbf{r}}\cdot d\mathbf{m})\hat{\mathbf{r}} = M\pi a^2 dz_S\, a^2 / r^2\hat{\mathbf{x}}$ and:

$$\mathbf{B}_{T,2}(y,z) = \frac{3\mu_0 M\,\pi a^4}{2}\int_{-L/2}^{L/2}\frac{dz_S}{[a^2 + y^2 + (z - z_S)^2]^{5/2}}\hat{\mathbf{x}} \tag{31}$$

$$\mathbf{B}_{T,2}(y,z) = \frac{\mu_0 M\,a^4}{2(y^2 + a^2)^2}\left(\frac{3(y^2 + a^2)(L/2 - z) + 2(L/2 - z)^3}{[(L/2 - z)^2 + y^2 + a^2]^{3/2}} + \frac{3(y^2 + a^2)(L/2 + z) + 2(L/2 + z)^3}{[(L/2 + z)^2 + y^2 + a^2]^{3/2}}\right)\hat{\mathbf{x}} \tag{32}$$

The total magnetic field is: $\mathbf{B}_T(y,z) = \mathbf{B}_{T,1}(y,z) + \mathbf{B}_{T,2}(y,z)$, which can be written in a compact form as:

$$\mathbf{B}_T(y,z) = \frac{\mu_0 M}{2(1 + \bar{y}^2)^2}\sum_{n=1,2}\frac{\bar{w}_n[(1 - \bar{y}^2)(\bar{y}^2 + \bar{w}_n{}^2) + 2]}{(1 + \bar{y}^2 + \bar{w}_n{}^2)^{3/2}}\hat{\mathbf{x}} \tag{33}$$

where the subscript $T$ refers to "trap", $\bar{y} = y/a$ and $\bar{w}_1 = (L/2 + z)/a$ and $\bar{w}_2 = (L/2 - z)/a$.

**<u>Special Case: Center of the Trap ($x$ = 0, $z$ = 0)</u>**

A special case can be obtained at the center of the trap ($x$ = 0, $z$ = 0), Eq. 33 can be simplified into:

$$\mathbf{B}_T(y,0) = \mu_0 M \frac{\bar{L}\left[(1-\bar{y}^2)(\bar{L}^2+4\bar{y}^2)+8\right]}{(1+\bar{y}^2)^2(\bar{L}^2+4\bar{y}^2+4)^{3/2}}\hat{\mathbf{x}} \tag{34}$$

where $\bar{L} = L/a$. In the long magnet limit ($\bar{L} \to \infty$) this reduces to a simple expression:

$$\mathbf{B}_{T\infty}(y,0) = \mu_0 M \frac{1-\bar{y}^2}{(1+\bar{y}^2)^2}\hat{\mathbf{x}} \tag{35}$$

### *A.4. Comparison of various models*

**Exact model: Magnetic Scalar Potential vs. Vector Potential (Bound Surface Current)**

The exact magnetic field models that we derived in Section A.1 and A.2 are for a single diametric magnet. To form our magnetic trap we place two identical magnets centered at ($\pm a$, 0, 0) as shown in the inset of Figure S4a. In this work, we will only need to consider the magnetic field at the center plane (i.e. $x = 0$). The total magnetic field for the trap in this center plane is given as:

$$\mathbf{B}_T(y,z) = \mathbf{B}_M(a,y,z) + \mathbf{B}_M(-a,y,z) \tag{36}$$

where $\mathbf{B}_M$ is the magnetic field from the scalar potential (Eq. 16) or vector potential model (Eq. 27). Note that $\mathbf{B}_T$ has only $x$ component due to the pair symmetry of the magnets.

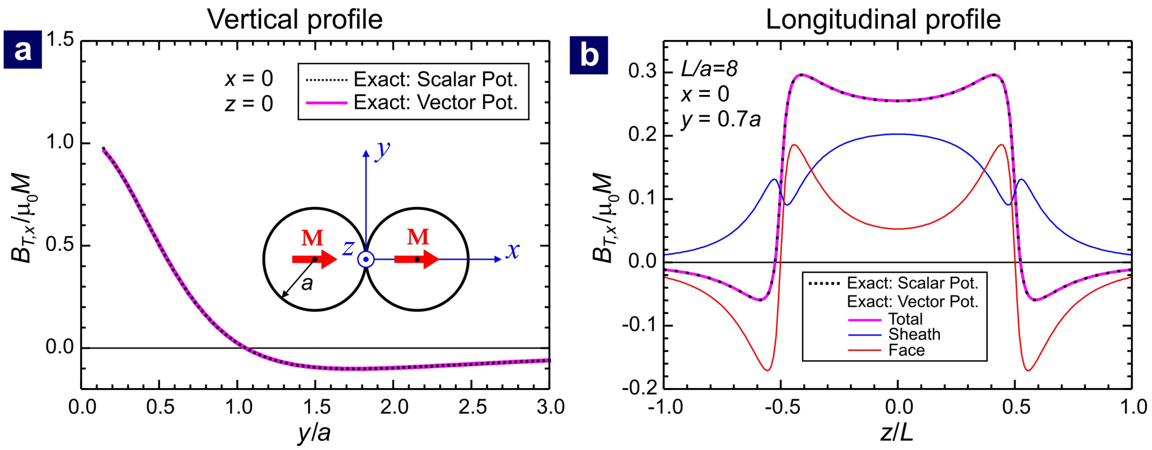


**Figure S4. Comparison of scalar and vector potential magnetic field model.** The magnetic field is calculated (as dimensionless quantity $B/\mu_0 M$) at the center of the trap ($x = 0$): (**a**) Along $y$-direction at the center ($z = 0$). (**b**) Along the longitudinal $z$-direction at $y = 0.7a$. The vector potential/surface current model allows us to decompose the sheath ($B_S$) and face ($B_F$) contribution.

We implement the magnetic field calculation for both models numerically and compare them as shown in Figure S4. *They both yield identical results*, except with the magnetic vector potential model we can decompose the sheath and face contribution as shown Figure S4b.

**PDL vs. Exact model:**

We can make similar comparison for the "PDL" model versus the "Exact" model (e.g. scalar potential model in Eq. 16 and 36) as shown in Figure S5. First, along the vertical ($y$) direction, the PDL model produces excellent agreement with the "Exact" model. We only start to observe some discrepancy at very short magnet length i.e. $L/a \le 2$. Along longitudinal direction the PDL model produces reasonable agreement only for long magnets. Near the edge of the magnet, the PDL model indeed reproduces the camelback hump albeit with some discrepancy as it fails to account the exact contribution from the end faces of the magnet. Nevertheless the PDL model produces very good approximation at the center of the trap where $z/L \sim 0$.

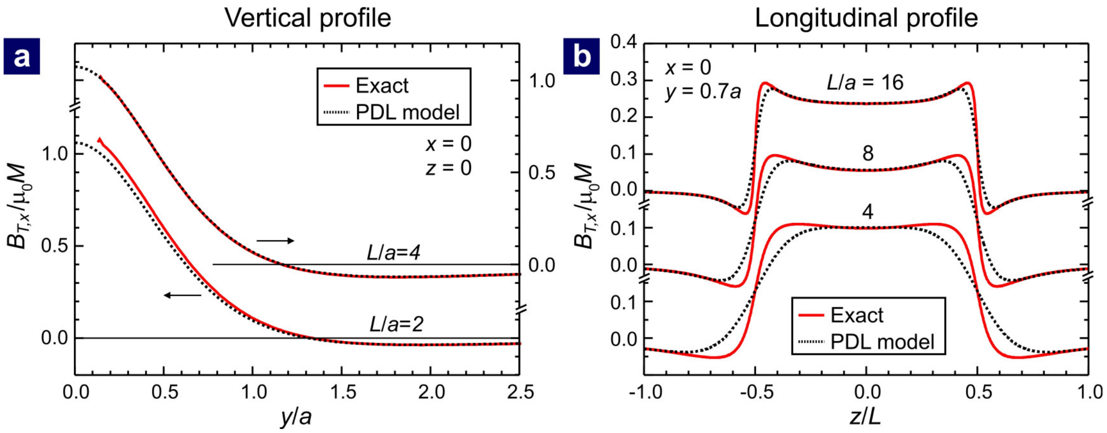


**Figure S5. Comparison of the "Exact" (scalar potential) and PDL model.** The magnetic field is calculated at the center plane ($x = 0$) and with varying magnet aspect ratio $L/a$: (**a**) Along $y$-direction at the center ($z = 0$). (**b**) Along the longitudinal direction at $y = 0.7a$.

## *B. The Magnetization of the Rod*

In the presence of magnetic field the trapped rod will get magnetized. We will derive the magnetic field **B** and **H** for a long cylinder with radius $a$ and uniform magnetization $M$ perpendicular to its axis [26]. Since there is no current in the cylinder, we can use $\nabla \times \mathbf{H} = 0$ and, similar to section II.A.1, we define a magnetic scalar potential such that $\mathbf{H} = -\nabla\Phi_M$. In cylindrical coordinate, the scalar potential can be written as: $\Phi_M = \Phi_M(r,\theta)$.

The magnetostatic boundary condition requires:

$$\mathbf{H}_r(r=a^+) - \mathbf{H}_r(r=a^-) = -\frac{\partial\Phi_M(r=a^+)}{\partial r} + \frac{\partial\Phi_M(r=a^-)}{\partial r} = \hat{\mathbf{r}}\cdot\mathbf{M} \tag{37}$$

This equation yields:

$$\Phi_M(r,\theta) = \frac{M}{2} r\cos\theta \text{ for } r < a, \quad \text{and} \qquad \Phi_M(r,\theta) = \frac{M}{2}\frac{a^2}{r}\cos\theta \text{ for } r > a \tag{38}$$

$$\mathbf{H} = -\frac{\mathbf{M}}{2} \text{ for } r < a; \text{ and } \qquad \mathbf{H} = \frac{Ma^2}{2r^2}\left(\cos\theta\,\hat{\mathbf{r}} + \sin\theta\,\hat{\boldsymbol{\theta}}\right) \text{ for } r > a. \tag{39}$$

Now we can calculate the magnetization induced on a rod by a magnetic field perpendicular to its axis. The magnetic field inside the cylinder can be written as: $\mathbf{B}_R = \mu_0(\mathbf{H}_R + \mathbf{M}_R)$ and from Eq. 39, we have $\mathbf{B}_R = \mu_0\mathbf{M}_R/2$. Using the relation $\mathbf{B}_{\text{tot}} = (\chi+1)\mu_0\mathbf{H}_{\text{tot}}$, we have: $\mathbf{B} + \mu_0\mathbf{M}_R/2 = (\chi+1)\left(\mathbf{B} - \mu_0\mathbf{M}_R/2\right)$.

Finally, the magnetization of the rod due to applied magnetic field $B$ is:

$$\mathbf{M}_R = \frac{2\chi}{\mu_0(\chi+2)}\mathbf{B} \tag{40}$$

## *C. The Vertical (y) Confinement*

We investigate the vertical confinement issue and the equilibrium position of the rod. The total potential energy of the trapped rod including gravity can be written as:

$$U_T(x,y,z) = V_R(\rho g y - \mathbf{M}_R \cdot \mathbf{B}_T) = V_R\left(\rho g y - \frac{2}{\mu_0}\frac{\chi}{\chi+2}B_T{}^2(x,y,z)\right) \tag{41}$$

The potential profile along the vertical direction is plotted in Figure S6a. At the center of the trap ($x$ = 0 and $z$ = 0), the equilibrium point $\bar{y}_0$ occurs when $F_y = -\partial U_T/\partial y = 0$ :

$$F_y = -V_R\left(\rho g + \frac{\mu_0 M^2}{a}\frac{\chi}{\chi+2}f_{\text{Y}}(\bar{y}_0,\bar{L})\right) = 0, \text{ or } \qquad -\frac{\rho g\, a}{\mu_0 M^2}\frac{\chi+2}{\chi} = f_{\text{Y}}(\bar{y}_0,\bar{L}) \tag{42}$$

where:

$$f_{\text{Y}}(\bar{y},\bar{L}) = -2a/\mu_0{}^2 M^2 \times \partial B_T{}^2(y,0)/\partial y \tag{43}$$

is a dimensionless geometrical prefactor function proportional to the diamagnetic repulsion force in $y$-direction. This can be calculated using the "Exact" magnetic field model (Section II.A.1) or the PDL model as shown below:

$$f_{\text{Y}}(\bar{y},\bar{L}) = \frac{8\bar{y}\,\bar{L}^2[(\bar{y}^2-1)(4\bar{y}^2+\bar{L}^2)-8][\bar{L}^4(\bar{y}^2-3)+10\bar{L}^2(\bar{y}^2-3)(1+\bar{y}^2)+24(\bar{y}^2-4)(1+\bar{y}^2)^2]}{(1+\bar{y}^2)^5(\bar{L}^2+4\bar{y}^2+4)^4} \tag{44}$$

In long magnet limit ($\bar{L} \to \infty$), this expression can be simplified as $f_Y(\bar{y}, \bar{L}) \simeq f_{Y\infty}(\bar{y})$ where:

$$f_{Y\infty}(\bar{y}) = \frac{8\bar{y}(3-\bar{y}^2)(1-\bar{y}^2)}{(1+\bar{y}^2)^5} \tag{45}$$

The plot of this function is shown in Figure S6b. Note that this function has maximum of $f_{Y,max}$ = 4.138 at $\bar{y} = 0.287$ which limit the availability of solutions. For $\bar{y} > 0$ it has three roots at 0, 1 and $\sqrt{3}$. For diamagnetic material ($\chi < 0$), the left hand side in Eq. 42 is always positive; therefore this equation would only yield solutions for:

$$0 < \bar{y} < 1 \text{ or } \bar{y} > \sqrt{3} \tag{46}$$

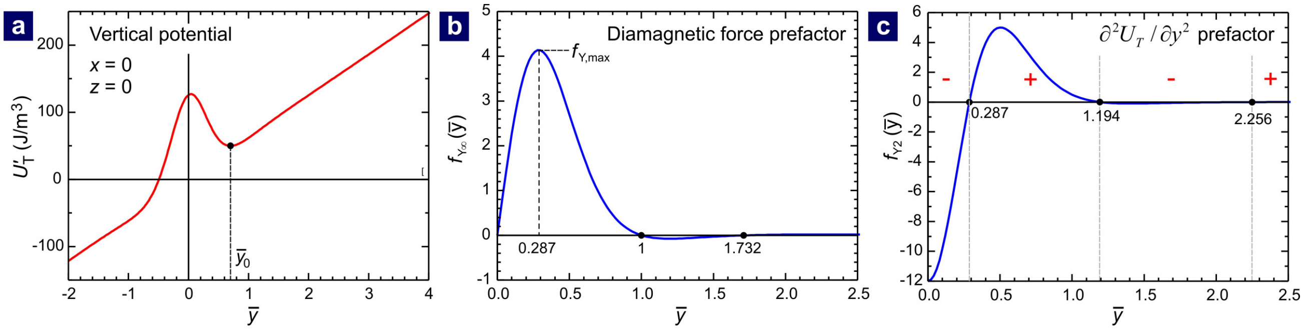


**Figure S6. Vertical confinement study**: (**a**) The vertical potential (per unit rod volume) as a function of normalized height $\bar{y} = y/a$. (**b**) The diamagnetic force prefactor function $f_{Y\infty}(\bar{y})$. (**c**) $f_{Y2}(\bar{y})$ plot to evaluate the stability condition.

In order for the system to be in stable equilibrium: $\partial^2 U_T / \partial y^2 > 0$, this gives:

$$-2\frac{\chi}{\chi+2}\mu_0 M^2 V_R f_{Y2}(\bar{y}) > 0; \text{ or } \qquad f_{Y2}(\bar{y}) > 0 \tag{47}$$

where $f_{Y2}(\bar{y}) = 4(5\bar{y}^6 - 33\bar{y}^4 + 39\bar{y}^2 - 3)/(1+\bar{y}^2)^6$ is the prefactor function for $\partial^2 U_T / \partial y^2$ for long magnet limit. The plot of $f_{Y2}(\bar{y})$ is shown in Figure S6c and for $\bar{y} > 0$, it has three roots at: 0.287, 1.194 and 2.256. A stable levitation only occurs for $f_{Y2}(\bar{y}) > 0$ at:

$$0.287 < \bar{y} < 1.194 \qquad \text{or} \qquad \bar{y} > 2.256 \tag{48}$$

Combining Eq. 46 and 48 we have the final condition for stable levitation:

$$0.287 < \bar{y} < 1 \qquad \text{or} \qquad \bar{y} > 2.256 \tag{49}$$

The first condition: $0.287 < \bar{y} < 1$ is more likely to be achieved compared to the second as $f_Y(\bar{y})$ is very small in the range of $\bar{y} > 2.256$ that severely limit the availability of solutions. In this range, in order to yield a solution for equilibrium height, we should have:

$$-\frac{\rho g a}{\mu_0 M^2}\frac{\chi+2}{\chi} < f_{Y,max} \tag{50}$$

From Figure S6b we have $f_{Y,max}$ = 4.138, thus in order the levitation to occur this condition sets the minimum $|\chi|$:

$$|\chi|_{min} = \frac{2}{1+f_{Y,max}\,\mu_0 M^2/\rho g a} \tag{51}$$

Thus levitation can be more easily achieved with rod that is more diamagnetic (more negative $\chi$) and lower density; or with magnets with stronger magnetization but smaller radius.

## Finite Magnet Length Consideration:

We can repeat the analysis above for a more general case where $L$ is finite. Here we use the "Exact" model from Section II.A.1 (Eq. 16 and 36). The minimum diamagnetic susceptibility $|\chi|_{min}$ depends on $f_{Y,max}$ and we calculated these parameters against different $L/a$ and plot $|\chi|_{min}$ as shown below. Interestingly we observe that $|\chi|_{min}$ does not change much with the magnet aspect ratio $L/a$.

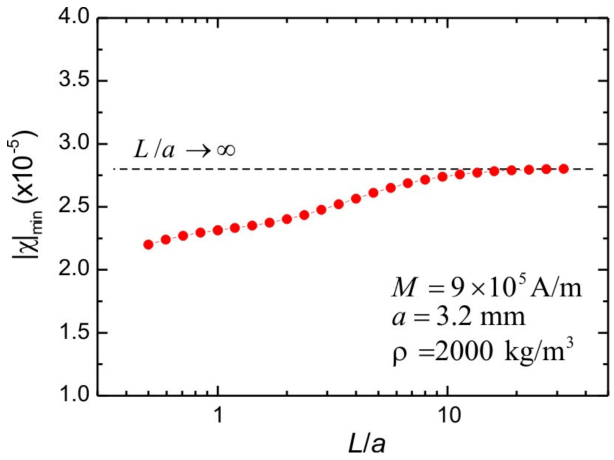


**Figure S7. $|\chi|_{min}$ at various magnet aspect ratio *L/a*.** The dashed line is the $|\chi|_{min}$ in the long magnet limit.

## *D. The Longitudinal (z) Confinement (Camelback Potential)*

The camelback potential experienced by the cylindrical diamagnetic rod levitated at height $y_0$ along the longitudinal ($z$) direction at the center of the trap ($x = 0$) can be written as:

$$U_M'(0, y_0, z) = -\frac{2\chi}{\mu_0(\chi+2)} B_T^{\,2}(y_0, z) \tag{52}$$

where $U_M' = U_M / V_R$ is the energy potential per unit rod volume. We ignore the gravitational potential contribution since $y_0$ is constant. We can use the "Exact" magnetic field expression (Eq. 1 and 36) as plotted in Figure 2b or we can use the PDL model (Eq. 33).

We provide some quantitative detail for the camelback humps in terms of its barrier height ($\Delta U_M'$) and the peak position ($z_P$) as shown in Figure S8a. Using the PDL model we can obtain analytical expressions and reasonable estimate of these quantities. We can solve for the camelback hump peak position $z_P$ by assuming $L >> \sqrt{a^2 + y_0^2}$ and obtain:

$$z_P = \pm(L/2 - \sqrt{2a^2 - y_0^{\,2}}) \tag{53}$$

We plot this $z_P$ (from the PDL model) vs. magnet aspect ratio $L/a$ in Figure S8a and compare it with the one derived using "Exact" model. We found that Eq. 53 provides a reasonable estimate for $z_P$, which is about 0.5$a$ less than the "Exact" model.

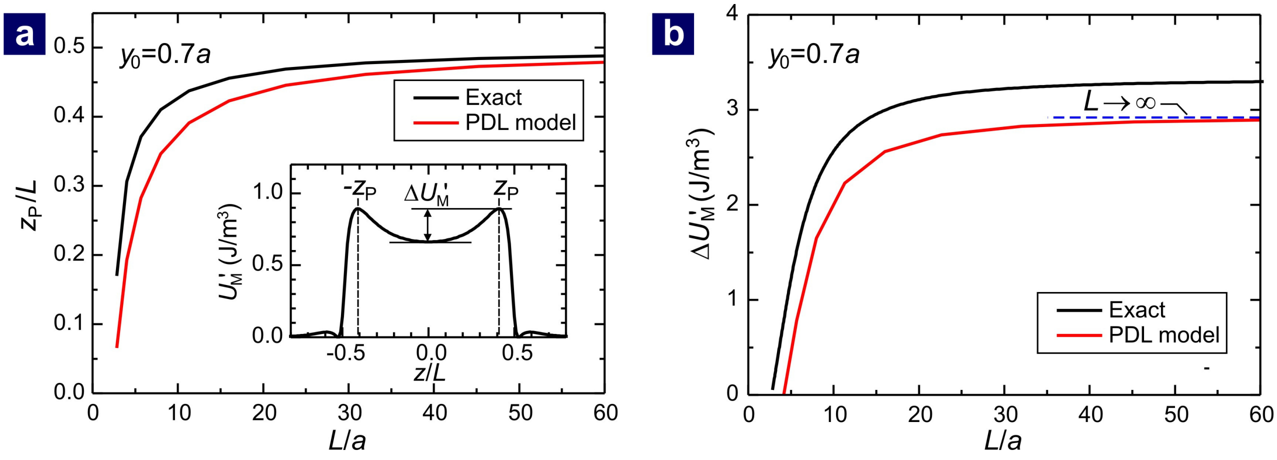


**Figure S8. Characteristics of the camelback peak and barrier height**. Using Exact and PDL model as a function of $L/a$: (**a**) Peak position $z_P$. **Inset:** Schematics of the camelback potential. **(b)** Barrier height $\Delta U_M'$. Dashed line: $\Delta U_M'$ using PDL model in the long magnet limit.

The camelback barrier height is given as:

$$\Delta U'_M = U'_M(0, y_0, z_P) - U'_M(0, y_0, 0) \tag{54}$$

Using the PDL model and long magnet limit ( $L \to \infty$ , Eq. 35), we can calculate the potential energy for the rod at the center (0, $y_0$, 0):

$$U'_M(0, y_0, 0) = -\frac{\chi}{2(\chi+2)}\mu_0 M^2 \left[\frac{2(1-\bar{y}_0^2)}{(1+\bar{y}_0^2)^2}\right]^2 \tag{55}$$

where $\bar{y}_0 = y_0 / a$. We ignore the gravitational potential contribution since $y_0$ is constant. The potential energy at the camelback peak (0, $y_0$, $z_P$) can be expressed as:

$$U'_M(0, y_0, z_P) = -\frac{\chi}{2(\chi+2)}\mu_0 M^2 \left[\frac{2(2-\bar{y}_0^2)^{3/2}}{3\sqrt{3}(1+\bar{y}_0^2)^2} + \frac{(1-\bar{y}_0^2)}{(1+\bar{y}_0^2)^2}\right]^2 \tag{56}$$

Therefore we can obtain the barrier height for the long magnet limit as:

$$\Delta U'_M = -\mu_0 M^2 \frac{\chi}{2(\chi+2)}\left[\left(\frac{2(2-\bar{y}_0^2)^{3/2}}{3\sqrt{3}(1+\bar{y}_0^2)^2} + \frac{(1-\bar{y}_0^2)^2}{(1+\bar{y}_0^2)^2}\right)^2 - \left(\frac{2(1-\bar{y}_0^2)}{(1+\bar{y}_0^2)^2}\right)^2\right] \tag{57}$$

This expression is plotted in Figure S8b (indicated as a dashed line) which is about 10% smaller than the value from the "Exact" model. We can also calculate $\Delta U'_M$ using the PDL model for any finite magnet length and compare them with the "Exact" model calculation as shown in Figure S8b. We find that the PDL model provides reasonable rough estimate for $\Delta U'_M$ .

## E. The Lateral (x) Confinement and Comparison

In $x$-direction, the rod is flanked by the two magnets. We can calculate the lateral potential confinement along the $x$-axis using Eq. 41 around the equilibrium point (0, $y_0$, 0). Away from the center plane ($x$ = 0), the magnetic field also possesses $y$ component besides $x$ component. Thus the total magnetic field along $x$-direction is given as: $B_T{}^2(x, y_0, 0) = B_{T,x}{}^2(x, y_0, 0) + B_{T,y}{}^2(x, y_0, 0)$ where $y_0$ is the equilibrium height position.

We can compare this lateral confinement potential in ($x$) direction with those from other directions ($y$ and $z$ as have been discussed in Section C and D). These confinement potentials are plotted on the same spatial scale in Figure S9. It is clear that the confinement along the $z$ direction (the camelback potential) is the weakest. This fact is also evident, if we compare the "spring constant" from each

direction i.e. $k_i = \partial^2 U_T / \partial i^2$ where $i = x$, $y$ or $z$. In our example we have: $k_x : k_y : k_z = 376$: 1,117 : 1, which shows that $k_z$ is the smallest among three.

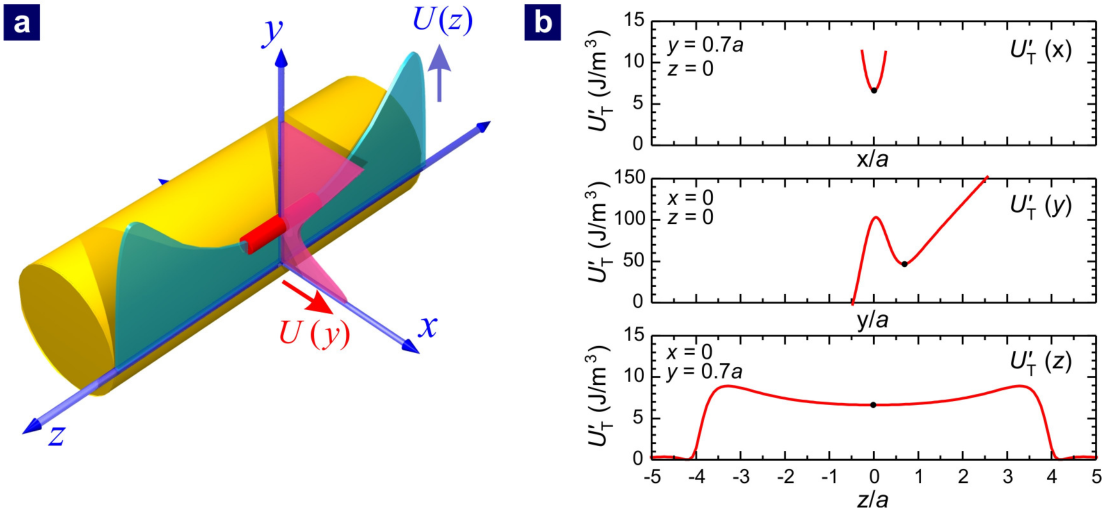


**Figure S9. The confinement potentials along all directions ($x$, $y$ and $z$).** (**a**) Schematic diagram of the confinement potentials. (**b**) The confinement potential profile (per unit rod volume) along $x$, $y$ and $z$ axis near the equilibrium point (0, $y_0$, 0) (magnet: $M = 9\times10^5$ A/m, $L/a = 8$ and graphite rod: $\chi = -10^{-4}$ ) .

## *F. The Oscillation in the Camelback Potential*

To describe the oscillation of the rod along the camelback potential we use the following approximations: (1) Small diameter rod ($b \ll a$) so that the magnetic field can be considered uniform in the radial extent of the rod; and (2) Short rod approximation ($l \ll L$) so that the potential experienced by the rod can be considered parabolic. Experimentally, the stability condition also dictates that $l > l_{\min}$ so that the rod still levitates.

We can approximate the center of the camel back potential with a parabolic potential $\Delta U_Z(z) = \frac{1}{2} k_z z^2$ for a small oscillation amplitude ($\ll L$) where $k_z$ is the potential "spring constant". We use Taylor's expansion:

$$U_T(0, y_0, z) = U_T(0, y_0, 0) + \frac{1}{2}\frac{\partial^2 U_T(0, y_0, 0)}{\partial z^2} z^2 \qquad \text{and} \qquad k_z = \frac{\partial^2 U_T(0, y_0, 0)}{\partial z^2} \tag{58}$$

Note that since $U_T$ is an even function of $z$ the first order term $\partial U_T / \partial z$ is zero. We have:

$$k_z = -\frac{V_R \mu_0 M^2}{L^2} \frac{\chi}{\chi + 2} f_{Z2}(\bar{y}_0, \bar{L}) \text{ , where} \tag{59}$$

$$f_{Z2}(\bar{y}, \bar{L}) = \frac{2L^2}{\mu_0{}^2 M^2} \frac{\partial^2 B_T{}^2(0, y, 0)}{\partial z^2} \tag{60}$$

is a dimensionless geometrical prefactor function proportional to the spring constant $k_z$.

This function can be calculated based on the "Exact" model (section II.A.1, Eq. 16 and 36) or alternatively we could obtain an analytical approximation using the PDL model (II.A.3):

$$f_{Z2}(\bar{y}, \bar{L}) = \frac{192\bar{L}^4(\bar{L}^2 + 4\bar{y}^2 - 16)[(\bar{L}^2 + 4\bar{y}^2)(1 - \bar{y}^2) + 8]}{(1 + \bar{y}^2)^2(4 + \bar{L}^2 + 4\bar{y}^2)^5} \tag{61}$$

In this parabolic potential, the rod can perform harmonic oscillation with angular frequency:

$$\omega^2 = \frac{k_Z}{m} = -\frac{\mu_0 M^2}{\rho} \frac{\chi}{\chi + 2} \frac{f_{Z2}(\bar{y}_0, \bar{L})}{L^2} \tag{62}$$

Since $T_z = 2\pi/\omega$ , we have:

$$\chi = -\frac{2}{1 + \mu_0 M^2 f_{Z2}(\bar{y}_0, \bar{L}) T_z^2 \big/ 4\pi^2 \rho L^2} \tag{63}$$

To calculate the magnetic susceptibility, we need to know the equilibrium height $y_0$. Fortunately, $T_z$ can be determined from $y_0$ and vice versa. From the vertical confinement analysis (Eq. 42) we have:

$$\frac{\mu_0 M^2}{\rho} \frac{\chi}{(\chi + 2)} = -\frac{ga}{f_Y(\bar{y}_0, \bar{L})} \tag{64}$$

Combining this and Eq. 62 we have:

$$\omega^2 = \frac{ga}{f_Y(\bar{y}_0, \bar{L})} \frac{f_{Z2}(\bar{y}_0, \bar{L})}{L^2} \tag{65}$$

Finally we obtain:

$$T_z = f_T(y_0, a, L) = 2\pi \sqrt{\frac{L^2}{g\, a} \frac{f_Y(\bar{y}_0, \bar{L})}{f_{Z2}(\bar{y}_0, \bar{L})}} \tag{66}$$

Note that $T_z$ is directly related to $y_0$ only by the magnet geometrical factor $L$ and $a$, *i.e.* $T_z = f_T(y_0, a, L)$ and independent of $M$ and the properties of the trapped rod (ρ, $b$ and $l$).

## Experimental data:

We performed a series camelback oscillation experiments to determine the magnetic susceptibility of graphite rods. We investigate the size dependent effect (diameter and length) of the graphite rods to test the validity of our model calculation described above.

First we use short graphite rod ($l$ = 4.5 mm) with various diameters and in two different setups: $L/a$=4 and 8 (see Section I for detail parameters). The rod length $l$ = 4.5 mm is chosen as approximately the shortest rod that still can levitate and align well to the $z$-axis in both setups. For each rod diameters, we measure $\rho$ and $T_z$ then calculate the equilibrium height $y_0$ (Eq. 66) and $\chi$ (Eq. 63). $T_z$ is measured from small amplitude oscillation with $z_{max}$ < 2 mm. The results are shown in Table S2 below and are also plotted in Fig. 3b-d. We observe that for each setup, $\chi$ is practically independent of the rod diameter which is expected in our small diameter approximation i.e. the rod diameter should have no effect. For the setup $L/a$ = 8 and 4 we obtain the average $\bar{\chi}$ = $-(11.0\pm1.6)\times10^{-5}$ and $-(9.0\pm1.9)\times10^{-5}$ respectively which show good consistency of our model calculation. The slightly lower $\chi$ in the $L/a$=4 setup is suspected due to finite length effect of the rod as discussed next.

| **Setup** | **Sample** | **Diameter** | **Density** | **Osc. period** | **Equil. height** | **Equil. height (Calc.)** | **Suscep-tibility (Calc.)** |
|---|---|---|---|---|---|---|---|
| | | $2b$ (mm) ±0.02 | $\rho$ (gr/cm$^3$) ±0.07 | $T_z$ (s) ±0.020 | $y_0/a$ ±0.045 | $y_0/a$ ±0.023 | $-\chi$ ($\times10^{-5}$) ±1.8 |
| ***L/a*=8** | HB/0.3 | 0.36 | 1.73 | 1.376 | 0.739 | 0.778 | 10.6 |
| | HB/0.5 | 0.55 | 1.74 | 1.360 | 0.754 | 0.789 | 11.6 |
| | HB/0.7 | 0.69 | 1.65 | 1.365 | 0.749 | 0.785 | 10.7 |
| | HB/0.9 | 0.89 | 1.70 | 1.363 | 0.743 | 0.786 | 11.1 |
| ***L/a*=4** | HB/0.3 | 0.36 | 1.73 | 0.737 | 0.743 | 0.728 | 8.3 |
| | HB/0.5 | 0.55 | 1.74 | 0.729 | 0.761 | 0.741 | 9.0 |
| | HB/0.7 | 0.69 | 1.65 | 0.714 | 0.738 | 0.764 | 9.9 |
| | HB/0.9 | 0.89 | 1.70 | 0.730 | 0.751 | 0.739 | 8.7 |

**Table S2.** Magnetic susceptibility determination experiment for short graphite rod of various diameters ($l$ = 4.5 mm, type "HB"). The equilibrium height $y_0/a$ is both measured (e.g. from Fig. 1b) and calculated ("Calc.") based on $T_z$ and using Eq. 66.

We investigate the effect of the length of the rod $l$ as presented in Figure S10. For comparison we also plot the camelback potential on the same length scale. For the long magnet setup ($L/a$=8) we found that $T_z$ does not change significantly for short rods ($l$ < 10 mm) as expected from the short

rod approximation i.e. that the rod's length should have no effect and the potential profile can be considered harmonic. However for the short magnet setup (*L*/*a*=4) we observe strong dependence of $T_z$ with respect to the length with some indication that $T_z$ settles to some value at very short rod near $l_{\rm min}$. This could happen because the camelback potential is narrower (the humps are closer) thus the parabolic potential approximation becomes less valid. Nevertheless, the data from the shortest possible rod $l$ = 4.5 mm still yields $\chi$ close to that measured in the *L*/*a*=8 setup (Table S2) suggesting that the short rod approximation at this minimum length is still acceptable for *L*/*a*=4 setup. From the trend in Figure S10b, shorter rod will yield slightly smaller $T_z$ and thus larger $\chi$ leading to better agreement with the $\chi$ measured from the *L*/*a*=8 setup (see Table S2).

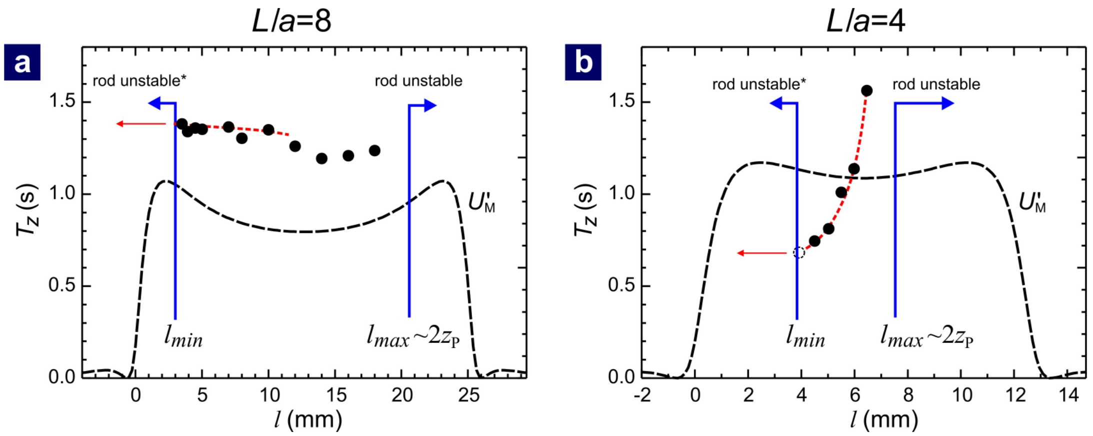


**Figure S10. Rod's length (*l*) effect to the oscillation period $T_z$.** Data for trap setup: (**a**) *L*/*a* = 8 (**b**) *L*/*a* = 4. The camelback potential (dashed curve) is also shown on the same *z* axis. Oscillation only occurs when the rod levitates ($l_{\rm min} < l < l_{\rm max}$). *Below $l_{\rm min}$ the rod becomes unstable i.e. it starts to tilt and touches the surface of the magnet. Red dashed curves are only for guide to the eyes.

## G. Underdamped Oscillation Analysis

We observe that the longitudinal oscillations always exhibit underdamped oscillation following $z_R(t) = A\exp(-t/\tau)\,\sin(\omega_d\, t+\phi)$, where $z_{\rm R}$ is the position of the rod's center (see Fig. 3a lower inset), $\tau$ is the damping time constant, $\omega_d$ is the "damped" angular frequency, $A$ is the initial amplitude and $\phi$ is the phase shift. When the damping effect is very strong ($\tau < T_z$), it will impact the measurement accuracy of the actual "undamped" period $T_z$. For the underdamped oscillation, the "undamped frequency" $\omega_0$ and the measured "damped frequency" $\omega_d$ are related as:

$$\omega_d^{\ 2} = \omega_0^{\ 2}\sqrt{1-\zeta^2} \qquad \text{where} \qquad \zeta = 1/\omega_0\tau \tag{67}$$

Therefore a damping effect will tend to reduce the observed oscillation frequency or increase the oscillation period. For $\chi$ measurement, it is necessary to obtain the "undamped" oscillation period $T_z$ from the "damped" oscillation period $T_{z,d}$. From Eq. 67 we obtain:

$$T_z = \frac{T_{z,d}}{\sqrt{1 + T_{z,d}^{\ 2} / (2\pi\tau)^2}} \quad (68)$$

Note that even for $\tau \sim T_z$ the error is rather small, about 1%, however since in some region $\chi$ is a strong function of $T_z$ (see Fig. 3d) – it is worthwhile to perform this correction to get more accurate $\chi$ measurement.

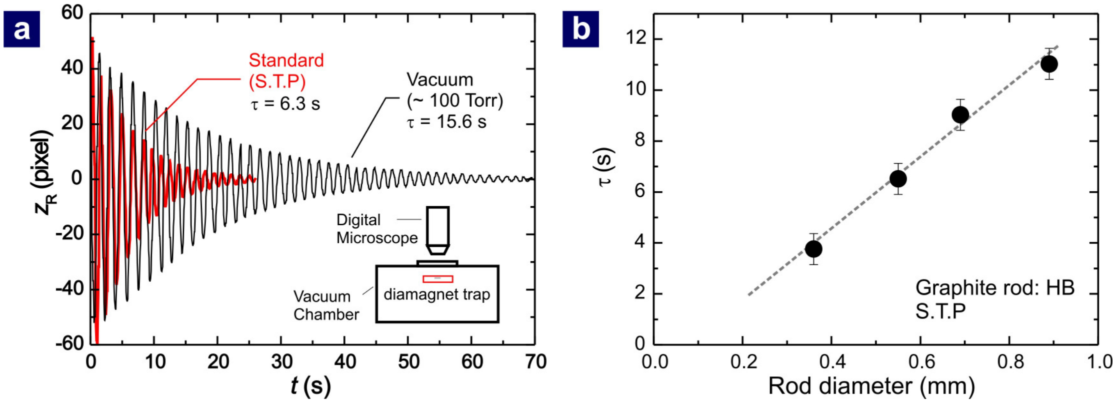


**Figure S11. Vacuum and diameter dependence test of underdamped oscillation:** (**a**) Vacuum test: Underdamped oscillation in standard temperature and pressure (S.T.P: 25 C and 760 Torr) vs. vacuum (~100 Torr) condition. (**b**) The damping time constant vs. rod diameter at S.T.P.

Now we discuss the origin of this damping effect, which could be attributed to: (1) air friction or viscosity effect; or (2) magnetic braking effect. Both are proportional to the velocity that could give rise to the underdamped behavior. The magnetic braking effect could be significant for a conductor moving in the presence of magnetic field. In our case, graphite is a rather good conductor (conductivity ~1/300 of copper) and the magnetic field at the center of the trap is relatively strong (~ 0.2 T at $\bar{y} \sim 0.7$, see Figure S4a) thus a magnetic braking effect could occur. To discriminate both effects we perform vacuum test and rod diameter test.

### (1) Vacuum test

We place the diamagnet trap system inside a vacuum chamber and capture the oscillation in the "standard" (chamber not pumped) and "vacuum" (chamber pumped to ~ 100 Torr) condition. When the pressure is very low it is expected that the air viscosity and damping effect will become weaker (or τ becomes longer). In contrast the magnetic braking effect should not depend on pressure. Our data in Figure S11a shows that the damping becomes significantly weaker in vacuum, thus this test suggests that the air friction effect dominates.

**(2) Rod diameter test**

Let us assume that both air friction and magnetic braking forces are present. We also assume that the rod is very short ($l$ ~ $2b$) so the air friction could be approximated by Stokes drag on a sphere, which is proportional to the radius $b$ given as:

$$F_S = -6\pi \mu_A b v \tag{69}$$

where $\mu_A$ is the viscosity of the air and $v$ is the velocity of the rod.

For the magnetic braking effect, the moving rod will induce eddy current distribution in the rod following:

$$\mathbf{J} = \sigma(\mathbf{E} + \mathbf{v} \times \mathbf{B}) \tag{70}$$

where σ is the conductivity of the rod. The term $\mathbf{v} \times \mathbf{B}$ is the electromotive term, **v** is the velocity vector and **E** is the build-up electric field that arises in the rod to maintain the continuity equation and boundary condition. The presence of **E** tends to weaken the overall eddy current. The magnetic braking force can be calculated as:

$$F_B = \int_V \mathbf{J} \times \mathbf{B}\, dV = -k_1 V_R \sigma B_x^{\ 2} v = -k_1 \pi b^2 l \sigma B_x^{\ 2} v \tag{71}$$

where $V_R$ is the rod's volume, and $k_1$ is a constant (<1) that accounts for the cancelling effect of the build-up electric field **E**. Note that if we ignore the boundary condition of the eddy current we have **E** = 0 everywhere in the rod and obtain $k_1 = 1$.

The total friction force is: $F_F = F_S + F_B = -(6\pi\mu_A b + k_1 \pi b^2 l \sigma B_x^{\ 2})v = -cv$, where $c$ is the coefficient of the viscous force. Following the analysis of underdamped oscillation we have:

$$\tau = \frac{2m}{c} = \frac{2\rho b l}{6\mu_A + k_1 \sigma B_x^{\ 2} b l} \tag{72}$$

where $m$ is the mass of the rod. If the air friction dominates, we will have: $\tau \simeq \rho b l / 3\mu_A$, which is proportional to the rod radius $b$. If the magnetic braking effect dominates: $\tau \simeq 2\rho / k_1 \sigma B_x^{\ 2}$, which is independent of $b$.

We repeated the oscillation analysis with several identical graphite rods (hardness "HB") of different diameters (nominally 0.3, 0.5, 0.7 and 0.9 mm) and plotted the damping time constant vs. rod diameter as shown in Figure S11b. The data shows that the damping time constant is proportional to the rod radius $b$, thus this test further confirms that the air friction effect dominates.

## *H. Custom-Designed 1D Potential System*

We could realize almost any arbitrary shape of 1D potential system by joining several segments of diametric magnet pairs with different magnetization *M*. The overall potential (per unit rod volume) is given as:

$$U'_M(z) = -\frac{2\chi}{\mu_0(\chi+2)}\sum_i B_{T,i}{}^2(0, y, z - z_i) \tag{73}$$

where $B_{T,i}(x, y, z)$ is the magnetic field of *i*-th segment which is proportional to the magnetization $M_i$ and $z_i$ is the center of the segment. For example, we could realize a double well and multiple well (superlattice) potential as shown below:

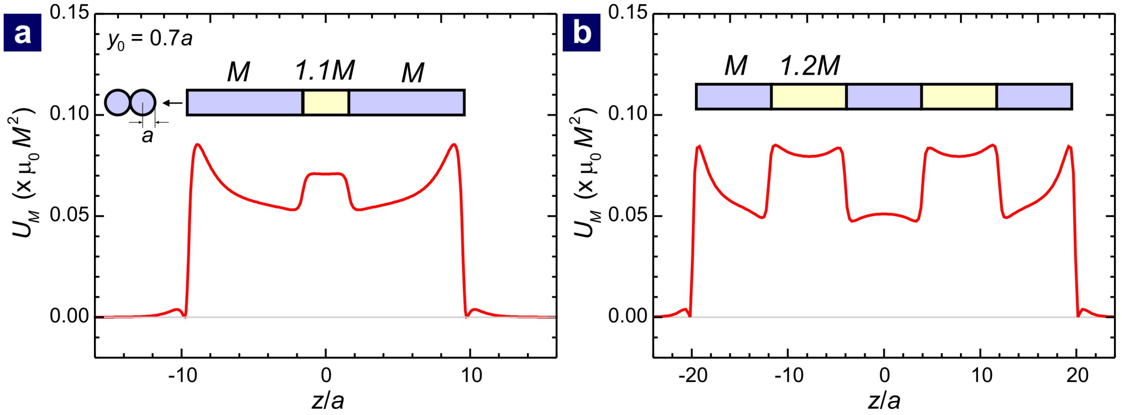


**Figure S12**. **Realization of various 1D potential:** (**a**) Double well (**b**) Multiple well. The relative magnetization of each segment is indicated in the schematic.

# References:

[24] J. D. Jackson, Classical Electrodynamics, (Wiley-VCH, New York, ed. 3, 1998).

[25] D. J. Griffiths, Introduction to Electrodynamics (Prentice Hall Upper Saddle River, NJ, ed. 3, 1999).

[26] K. McDonald, http://www.hep.princeton.edu/~mcdonald/examples/ph501set5.pdf
